# Supplementary material for: Strong Coupling of the Iron-Quadrupole and Anion-Dipole Polarizations in Ba(Fe$_{1-x}$Co$_x$)$_2$As$_2$
Source: arXiv:1401.3706 source file (2014-01-15)
Supplement: Supplementary file 1 [file SI2.pdf]

# [Supplementary Information] Strong coupling of the iron-quadrupole and anion-dipole polarizations in $Ba(Fe_{1-x}Co_x)_2As_2$

Chao Ma,[1,2] Lijun Wu,[1] Wei-Guo Yin,[1] Huaixin Yang,[2] Honglong Shi,[2] Zhiwei Wang,[2] Jianqi Li[2], C. C. Homes,[1] & Yimei Zhu[1]

[1]Condensed Matter Physics & Materials Sciences Department, Brookhaven National Laboratory, Upton, New York 11973, USA
[2]Beijing National Laboratory for Condensed Matter Physics, Institute of Physics, Chinese Academy of Sciences, Beijing 100190, China

## Technique details

### 1. Mapping the valence electron density

The $Ba(Fe_{1-x}Co_x)_2As_2$ single crystals (ref. S1) presented here have nominal $x$ = 0, 0.04, 0.06, 0.08, and 0.1 and $T_c$ = 0, 0, 12, 20, and 22.5 K, respectively.

The low-order electron structure factors was accurately measured by using CBED and then converted to the corresponding low-order x-ray structure factors by using the Mott-Bethe formula (ref. S2). The refined low-order electronic and x-ray structure factors are listed in Table S1, compared with the corresponding low-order x-ray structure factors in DFT and procrystal model (independent-atom model).

The experimental and calculated energy-filtered CBED pattern of 110 systematical row in $BaFe_2As_2$, shown in Figs. 1a and 1b of the main text, respectively, were taken from the sample of a refined thickness of 75.3 nm. Fig. 1c of the main text shows the line scan of the intensity profiles from the experimental and calculated patterns using the Bloch wave method (ref. S2). Five different systematic rows with small scattering angles were obtained, including 002, 200, 110, 011, and 013 reflections. The refined low-order electron and x-ray structure factors are listed in Table S1, compared with the corresponding low-order x-ray structure factors determined from DFT and the procrystal model. On the other hand, the high-order x-ray structure factors are dominantly contributed by atomic position and core charge, and in many cases they can be replaced by calculated structure factors from DFT electronic structure calculations or even procrystal, without losing significant accuracy.

We calculated the high-order x-ray structure factors based on density-functional theory (DFT) using the full potential linear augmented plane wave method implemented in WIEN2k software package (ref. S3). The muffin-tin radii $R_{\mathrm{mt}}$ were selected as 2.5, 2.2, and 2.1 a.u. for Ba, Fe/Co and As atoms, respectively. The maximum angular momentum of the radial wave functions ($l_{max}$) was chosen as 10 and $R_{\mathrm{mt}}K_{\mathrm{max}}$ was fixed at 7.0 to determine the basis size. The experimental lattice parameters (ref. S4) were used. Co substitution disorder was treated in virtual crystal approximation (VCA) and supercell approximation, which turns out to lead to essentially the same averaged electron density distribution, as presented in Fig. 2 of the main text. We tested a number of exchange correlation functionals, such as local density

approximation (LDA), generalized gradient approximation (GGA), and GGA+U (U = 1, 2, 3, and 4 eV). We found that they lead to the same conclusion.

Combining the accurately measured low-order and calculated high-order x-ray structure factors (the measured ones were adjusted to zero temperature by a temperature factor), the valence electron distribution and orbital occupancy were obtained through mutipole refinement (ref. S5) in consideration of the aspherical density model, in which 292 independent reflections without the multiplicity of crystal symmetry were used – we used the space group *I4/mmm* of the room-temperature crystal structure. Thus we can map out the charge density distribution.

For multipole refinement in the presence of the Co disorder, we follow the procedure of VCA used with WIEN2k. That is, for $Ba(Fe_{1-x}Co_x)_2As_2$, the atomic number (the charge number of the nucleus) of the Fe site is increased to $26 + x$ and the number of the valence electrons per Fe/Co atom is also increased by $x$. This is feasible because Co sits next to Fe in the periodic table and the core electrons of Co is basically the same as that of Fe. With only the core electrons being fix, all valence electrons are refined based on space group symmetry and experimental structure factors. The multipole refinement will adjust the valence electrons to fit the experimental structure factors. So the charge distribution we obtained is the symmetrically averaged distribution. Thus, we used this approach (in particular the same space group for all Co concentration levels) to investigate the average effects of Co doping. Since it is kind of similar to VCA, we shall refer to it as e-VCA ("experimentally"-VCA). Notably, they are expected to generate the similar Fe/Co charge monopole. However, there is a significant difference between e-VCA and VCA. In VCA, the crystal potential is averaged *before* theoretical calculations. In e-VCA, the realistic Fe and Co potentials are presented in the measurements; only the results are averaged by fitting to a model where the translational symmetry is preserved, i.e., e-VCA is a *posterior* treatment. Hence, with the replacement of the VCA low-order structure factors by the experimental ones, e-VCA would yield more realistic information, especially on electron correlation, than VCA. The results obtained from using e-VCA and GGA+VCA are compared below.

Figs. S1a and S1b show the experimental difference charge density map in the (100) and (110) planes for the parent compound $BaFe_2As_2$. They are well reproduced by the calculated difference charge density map obtained from using the GGA method (Figs. S1b and S1d).

As for the optimally doped case $x$=0.1, the calculated difference charge density map obtained from using the GGA+VCA method (Figs. S2b and S2d) fails to reproduce the experimental (e-VCA) one (Figs. S2a and S2c). Instead, the theoretical charge density map looks quite similar to the undoped case (Figs. S1b and S1d), indicating the rigid-band feature, in agreement with previous GGA+VCA calculations of the band structure. This means that the classic Fe/Co charge monopole-As charge dipole interaction (the averaged Fe/Co charge monopole remains unchanged upon Co doping, providing Ba and As remain 2+ and 3-, respectively) cannot yield the observed strong anion polarization. It follows that to detect the evolution of anion polarization with Co doping, the theoretical methods should be capable of capturing the physics of electron correlation and charge fluctuation beyond the widely used

local density approximation or generalized gradient approximation of DFT.

In hindsight, $Ba(Fe_{1-x}Co_x)_2As_2$ is the best system to reveal the strong nonlinearity of anion polarization, since the average value of the Fe/Co charge monopole remains unchanged upon Co substitution for Fe.

*A structural change effect?*—Since the structural change induced with Co doping is rather small, we ruled it out as a driving force for the observed large change in the electron redistribution by have performed the following DFT simulations: (i) The x=0.1 electron map with the x=0 structure and (ii) the x=0 electron map with the x=0.1 structure. No noticeable variation was observed as the structure changed.

*Charge doping versus isovalent substitution.*—Both our CBED and EELS results favor the picture that substituting Co for Fe effectively dopes charge carriers into the Fe planes. This is consistent with the traditional picture of nominal $Co^{3+}$ substitution for $Fe^{2+}$, which is also supported by a number of observations, such as changes in Hall constant (ref. 43 in the main text) and Fermi surface volume estimated from both ARPES experiments (ref. 37 in the main text) and DFT calculations (refs. 26,37,44,45 in the main text). By contrast, x-ray absorption near edge structure (refs. 46,47 in the main text) seemed to support the $Co^{2+}$ isovalent substitution picture (ref. 48 in the main text).

## 2. Phonon calculations

The *ab initio* calculations on $BaFe_2As_2$ (*I4/mmm* space group) were performed using the full potential linearized augmented plane wave method in the WIEN2K implementation [1]. The generalized gradient approximation (GGA) exchange correlation potential was used. The zone center lattice modes were determined from the direct method using a 1x1x1 supercell; a 9x9x3 k-point mesh and $R_{mt}k_{max}$=8.5 having been determined to yield excellent energy convergence. As a first step the unit cell dimensions are optimized with respect the total energy, then the atomic fractional coordinates are refined until the total force on each of the atoms is typically less than 0.1 mRy/au. To obtain a complete set of Hellmann-Feynman forces, a total of six independent displacements are required; we have considered symmetric displacements, resulting in 12 separate structures, with atomic displacements of 0.04 Å. After each structure has converged using the criteria that the total change in forces on each atom are less than 0.01 mRy/au, the residual forces are collected for each set of symmetric displacements and a list of the Hellmann-Feynman forces are generated. The cumulative force constants deconvoluted from the Hellmann-Feynman forces introduced into the dynamical matrix, which is then diagonalized to obtain the phonon frequencies, as well as the atomic displacements and intensities, shown in Table S2. From the point of view of the infrared-active in-plane $E_u$ modes, the substitution of different alkali earths (i.e., Ca for Ba) into this structure produces a change in the low frequency $E_u$ mode, which primarily involves the alkali earth, but does not influence the high-frequency $E_u$ mode, which involves only the Fe and As atoms.

**References**

S1. Ma, C., Yang, H. X., Tian, H. F., Shi, H. L., Lu, J. B., Wang, Z. W., Zeng, L. J., Chen, G. F., Wang, N. L. & Li, J. Q. Microstructure and tetragonal-to-orthorhombic phase transition of $A\mathrm{Fe_2As_2}$ ($A$=Sr, Ca) as seen via transmission electron microscopy. Phys. Rev. B **79**, 060506(R) (2009).

S2. Wu, L., Zhu, Y., Vogt, T., Su, H., Davenport, J. W., & Tafto, J. Valence-electron distribution in $MgB_2$ by accurate diffraction measurements and first-principles calculations. Phys. Rev. B **69**, 064501 (2004).

S3. Blaha, P., Schwarz, K., Madsen, G., Kvasnicka, D. & Luitz J. WIEN2K, an augmented plane wave + local orbital program for calculating crystal properties. Karlheinz Schwarz, Technical University, Wien, Austria (2001).

S4. Sefat, A. S., Jin, R., McGuire, M. A., Sales, B. C., Singh, D. J. & Mandrus, D. Superconductivity at 22 K in Co-doped $BaFe_2As_2$ crystals. Phys. Rev. Lett. **101**, 117004 (2008).

S5. Volkov, A., Macchi, P., Farrugia, L. J., Gatti, C., Mallinson, P., Richter, T. & Koritsanszky, T. XD2006 - A computer program package for multipole refinement, topological analysis of charge densities and evaluation of intermolecular energies from experimental and theoretical structure factors. (2006).

Table S1 | Measured electron structure factors using the CBED and x-ray structure factors converted from electron structure factors for $BaFe_2As_2$ and $BaFe_{1.8}Co_{0.2}As_2$. The calculated x-ray structure factors from DFT and procrystal (independent-atom model) for $BaFe_2As_2$ are also listed for comparison with the experimental ones.

| Reflection | Experiments | | | | Calculations | |
|---|---|---|---|---|---|---|
| | Electron structure factors | | X-ray structure factors | | DFT | Procrystal |
| | undoped | Co-doped | undoped | Co-doped | undoped | undoped |
| 0 0 2 | -4.05±0.39 | -3.92±0.31 | -25.34±0.10 | -25.05±0.08 | -25.286 | -24.886 |
| 0 1 1 | 6.42±0.29 | 6.46±0.40 | 27.06±0.21 | 26.73±0.29 | 26.832 | 26.965 |
| 0 0 4 | 16.17±0.43 | 16.48±0.57 | 85.76±0.43 | 85.01±0.57 | 84.224 | 84.365 |
| 0 1 3 | 29.98±0.33 | 30.68±0.27 | 196.77±0.41 | 195.38±0.33 | 194.210 | 194.140 |
| 1 1 0 | 16.74±0.21 | 16.81±0.30 | 117.27±0.29 | 116.79±0.41 | 117.179 | 116.942 |
| 2 0 0 | 34.11±0.28 | 33.92±0.28 | 253.15±0.77 | 254.14±0.78 | 252.073 | 252.959 |

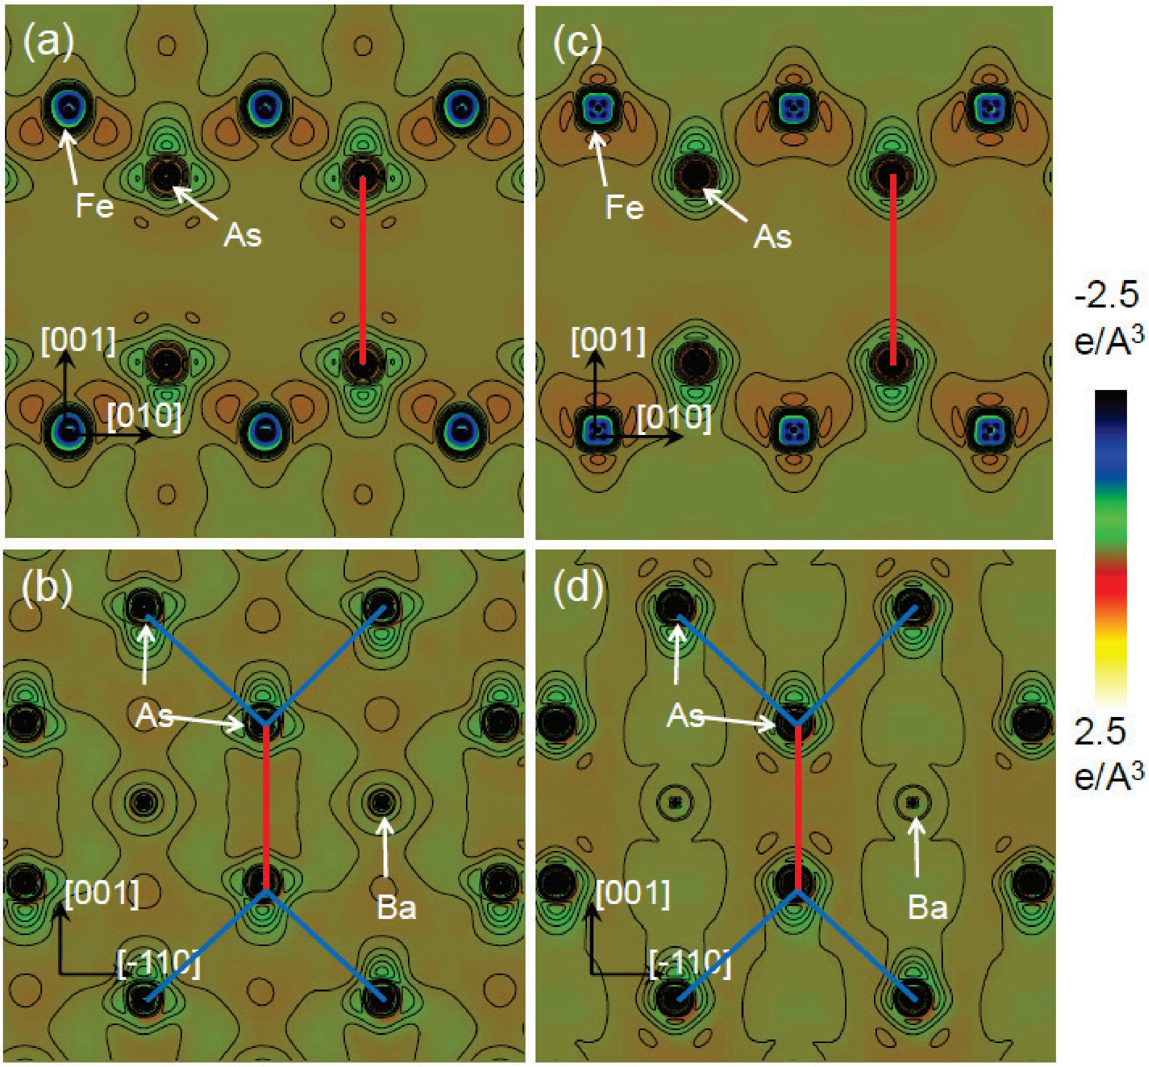


Figure S1 | **Difference density distribution in the undoped sample (*x*=0). a,** experiment in the (100) plane. **b,** experiment in the (110) plane. **c,** the calculated in the (100) plane. **d,** the calculated in the (110) plane. The color legend indicates the magnitude of the charge density and the contour plot has an interval of 0.05e/Å$^3$. The blue and red lines denote the As-As "bonding" in and between the FeAs layers, respectively. The experiment and theory data agree well.

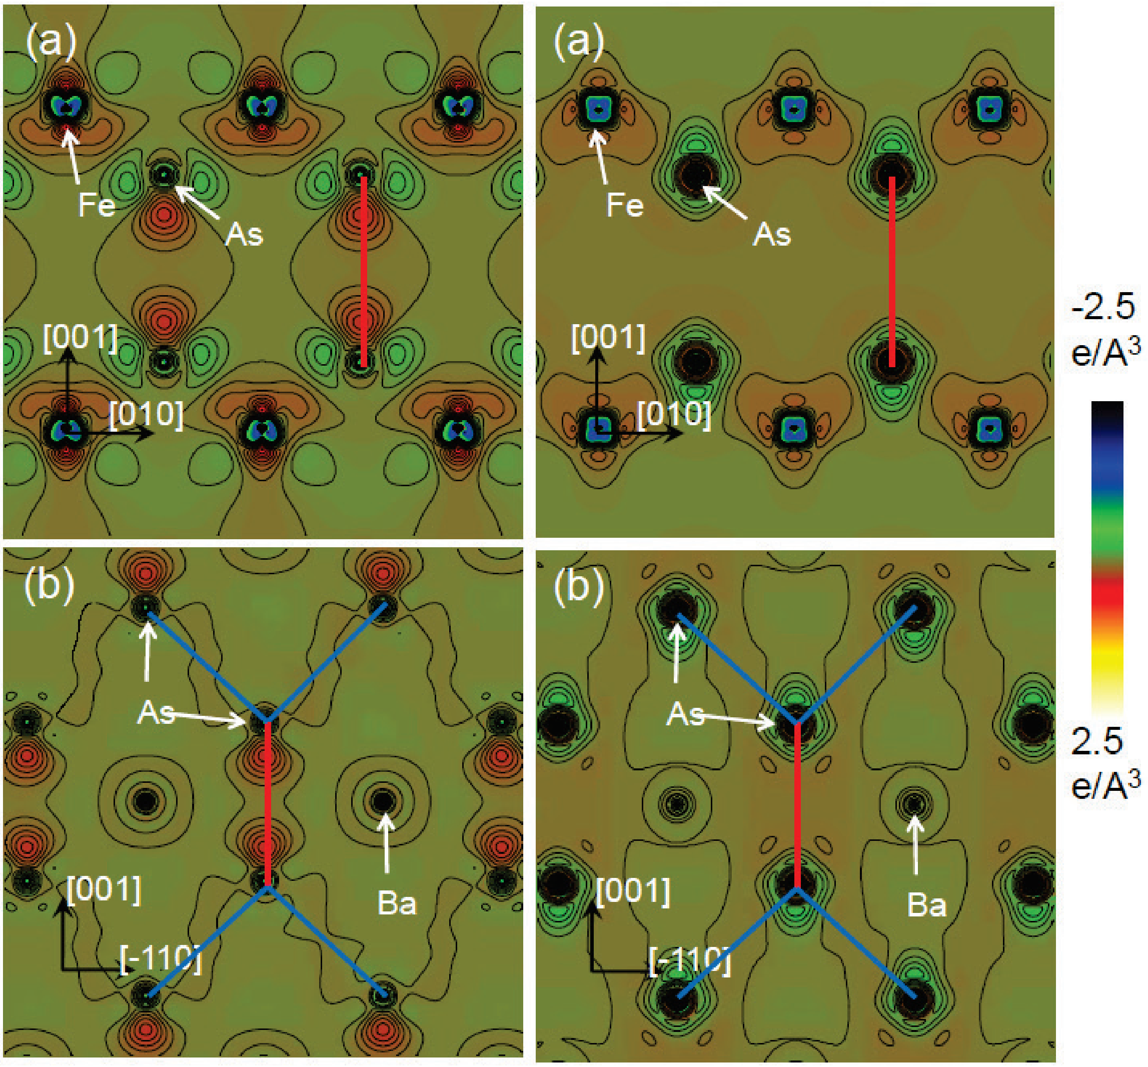


Figure S2 | **Difference density distribution in the optimally doped sample (*x*=0.1). a,** experiment in the (100) plane. **b,** experiment in the (110) plane. **c,** the calculated in the (100) plane. **d,** the calculated in the (110) plane. The blue and red lines denote the As-As "bonding" in and between the FeAs layers respectively. The color legend indicates the magnitude of the charge density and the contour plot has an interval of 0.05e/Å$^3$. Note that the charge density in between FeAs layers in the experimental map is much higher than that in the parent compound (Fig. S1), indicating stronger electronic polarization of the As anions, which cannot be reproduced by the GGA calculations.

Table S2 | Comparison of observed and calculated phonon frequencies (at room temperature) of the infrared and Raman active ($q$=0) modes for $BaFe_2As_2$ and $CaFe_2As_2$ in the tetragonal I4/mmm setting. The $A_{2u}$ and $E_u$ vibrations are infrared active along the $c$ axis and $a$-$b$ planes, respectively. The character of the modes is illustrated by the atomic intensities, shown to the first two significant figures.

$BaFe_2As_2$

| | | | Atomic Intensity | | |
|---|---|---|---|---|---|
| Symmetry | $\omega_{calc}$ ($cm^{-1}$) | $\omega_{obs}$ ($cm^{-1}$) | Ba | Fe | As |
| $E_g$ | 312 | | - | 0.72 | 0.28 |
| $E_u$ | 297 | 257 | - | 0.55 | 0.45 |
| $A_{2u}$ | 287 | | - | 0.58 | 0.42 |
| $B_{1g}$ | 236 | 215 | - | 1.00 | - |
| $A_{1g}$ | 207 | 181 | - | - | 1.00 |
| $E_g$ | 146 | | - | 0.29 | 0.71 |
| $E_u$ | 88 | 95 | 0.66 | 0.17 | 0.17 |
| $A_{2u}$ | 94 | | 0.66 | 0.14 | 0.20 |

$CaFe_2As_2$

| | | | Atomic Intensity | | |
|---|---|---|---|---|---|
| Symmetry | $\omega_{calc}$ ($cm^{-1}$) | $\omega_{obs}$ ($cm^{-1}$) | Ca | Fe | As |
| $E_g$ | 319 | | - | 0.78 | 0.22 |
| $E_u$ | 289 | 263 | - | 0.55 | 0.45 |
| $A_{2u}$ | 294 | | - | 0.56 | 0.44 |
| $B_{1g}$ | 215 | 208 | - | 1.00 | - |
| $A_{1g}$ | 214 | 189 | - | - | 1.00 |
| $E_g$ | 128 | | - | 0.22 | 0.78 |
| $E_u$ | 114 | 138 | 0.87 | 0.08 | 0.05 |
| $A_{2u}$ | 102 | | 0.87 | 0.07 | 0.06 |
